# Supplementary material for: Quasinormal-mode expansion of the scattering matrix
Source: arXiv:1609.03902 source file (2017-04-26)
Supplement: Supplementary file 1 [file supplementary.pdf]

# Supplemental Material: Quasinormal-mode expansion of the scattering matrix

Filippo Alpeggiani,[1,2] Nikhil Parappurath,[1] Ewold Verhagen,[1] and L. Kuipers[1,2]
[1]*Center for Nanophotonics, AMOLF, Science Park 104, 1098 XG Amsterdam, The Netherlands*
[2]*Kavli Institute of Nanoscience, Department of Quantum Nanoscience, Delft University of Technology, Lorentzweg 1, 2628 CJ Delft, The Netherlands*
(Dated: April 25, 2017)

Here, we provide additional data on the convergence of the quasinormal-mode expansion of the scattering matrix with respect to the choice of the number of modes. We consider the same example as Sec. IIB in the main text.

In Fig. S1, we illustrate the effect of including an additional pair of leaky modes to the set employed in Sec. IIB and originally displayed in Fig. 3(a) of the main text. The additional modes, which are highlighted with an arrow in Fig. S1(a), have been computed from the complex-frequency poles of the transmission amplitude with the Fourier modal method [Ref. 35 in the main text]. As it can be seen from Fig. S1(b), the agreement between the total transmission predicted from our theory (red solid curve) and the simulated data (dashed curve) is further improved with respect to Fig. 3(b) in the main text, in agreement with the considerations on the completeness of the quasinormal-mode basis.

Incidentally, we notice that other choices of the set of electromagnetic modes could provide comparable accuracy in the prediction of the transmission properties. For instance, in Fig. S1(c,d) we show that, in this particular example, excluding the modes with $\mathrm{Re}\,\tilde{\omega}_j < 0$ [see Fig. S1(c)] leads to an excellent agreement with the exact simulated data [Fig. S1(d)], without the need for including the additional pair of leaky modes discussed beforehand. The accuracy is probably due to the fact that the set of leaky modes in Fig. S1(c) is clearly symmetric with respect to the frequency range considered in Fig. S1(d), suggesting that, in some cases, the convergence behavior of the quasinormal-mode

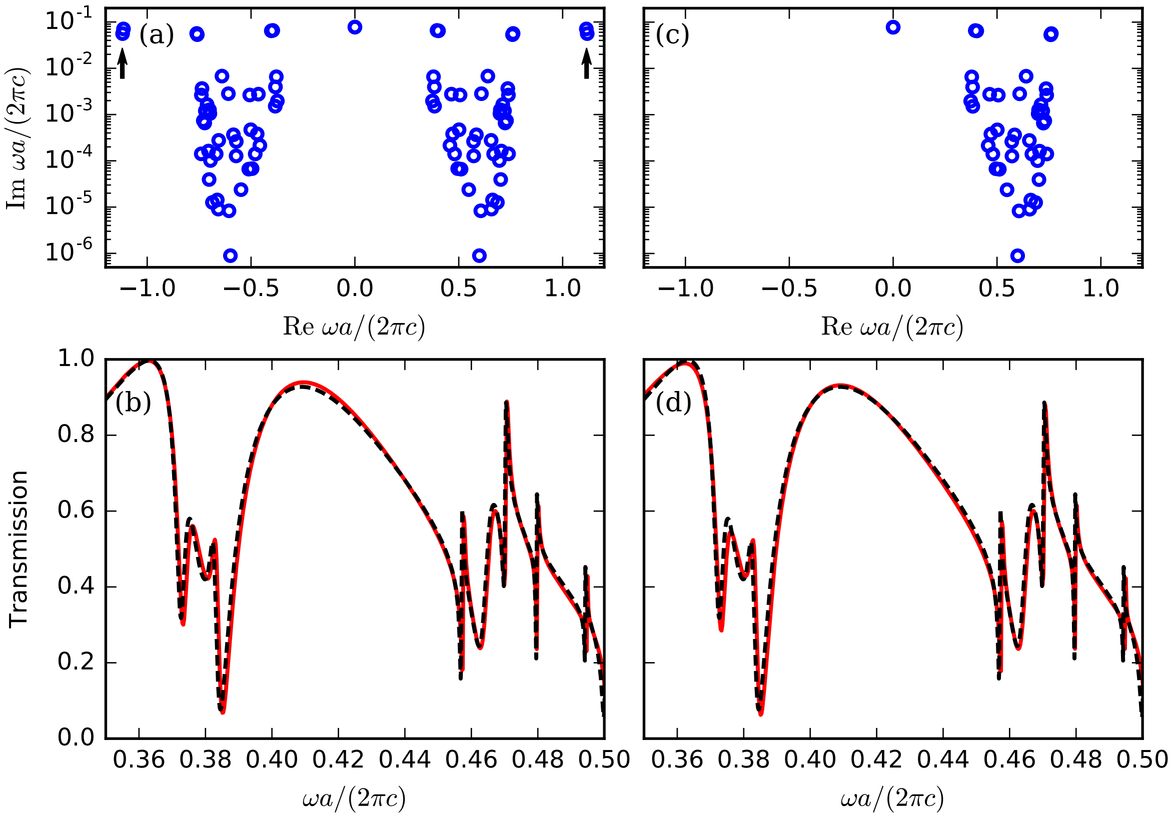


Figure S1. (a,c) Real and imaginary part (log scale) of different sets of the modal eigenfrequencies for the system considered in Sec. IIB in the main text. (b,d) Comparison of the total transmission computed by the quasinormal-mode expansion (solid red curve) with the exact result (dashed curve). Curves in (b) and (d) refer to the choices of the modes in (a) and (c), respectively.

expansion could be enhanced by a suitable choice of the modes.

For illustration purposes, we also show in Fig. S2(a,b) a plot of the amplitude of the electric field of two quasinormal modes selected from those of Fig. 3(a) in the main text, computed with the finite-element method. The corresponding complex frequencies are indicated in the figure. The plot displays a region of the $xz$ plane on the edge ($y = 0$) of the unit cell of the periodic photonic structure (see the schematic in Fig. 3(a) of the main text). The divergent behavior of the highly radiative quasinormal mode (b) is clearly recognizable.

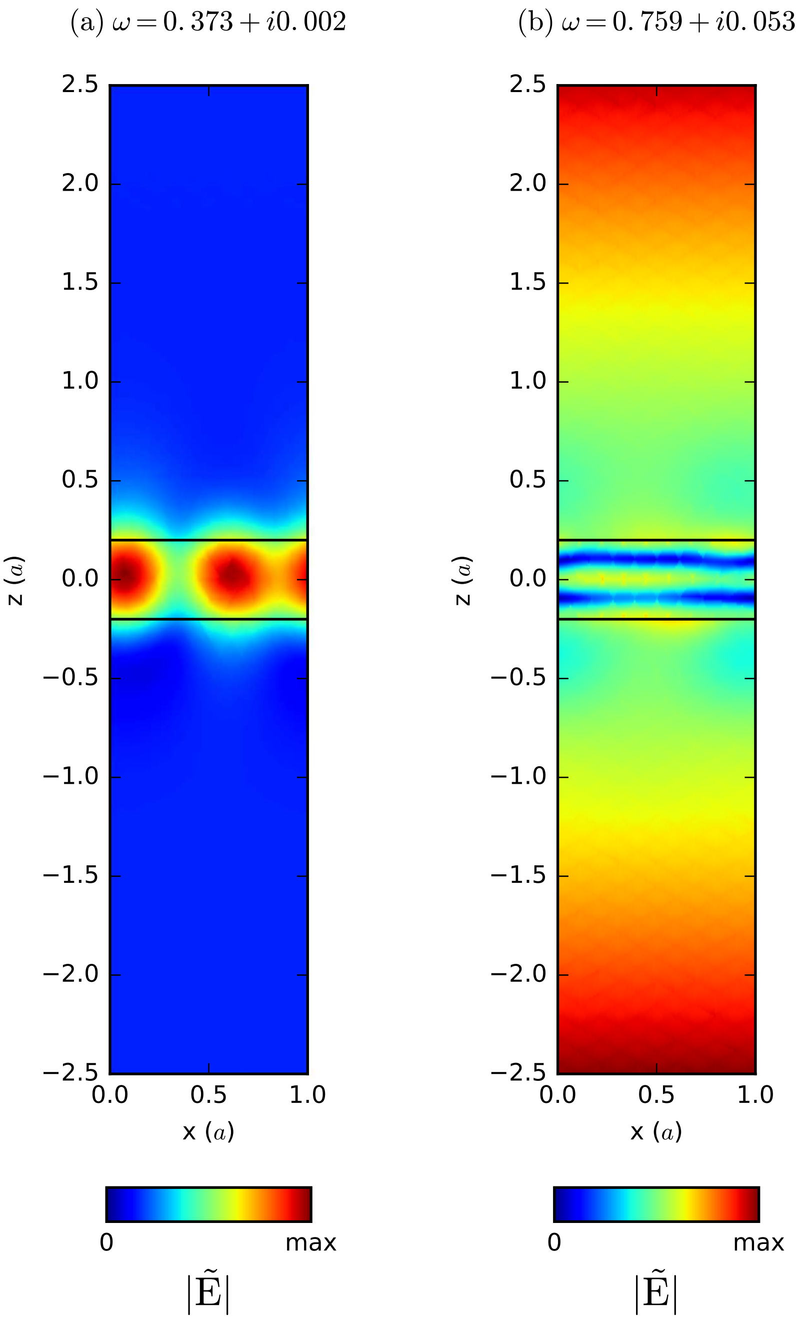


Figure S2. Amplitude of the electric field of two quasinormal modes selected from those of Fig. 3(a) in the main text. The plot shows a region of the $xz$ plane along the edge of the unit cell close to the long side of the L-shaped structure ($y = 0$). The complex frequencies of the modes are: (a) $\omega a/(2\pi c) = 0.373 + i0.002$, and (b) $\omega a/(2\pi c) = 0.759 + i0.053$.

In Fig. S3 we show the absorption cross section of the multilayered spherical nanoparticle of Fig. 5 in the main text (Sec. IID) for the cases of nonradiative Drude damping rates $\kappa_{\rm nr} = 0.01\omega_p$ and $\kappa_{\rm nr} = 0.04\omega_p$. The case $\kappa_{\rm nr} = 0.01\omega_p$ coincides with the results of Fig. 5 in the main text. In both cases, the results obtained with the quasinormal-mode expansion (solid lines) are compared with the exact generalized Mie theory (dashed lines). The plot shows a good agreement between the modal expansion and the exact theory even for larger dissipation rates.

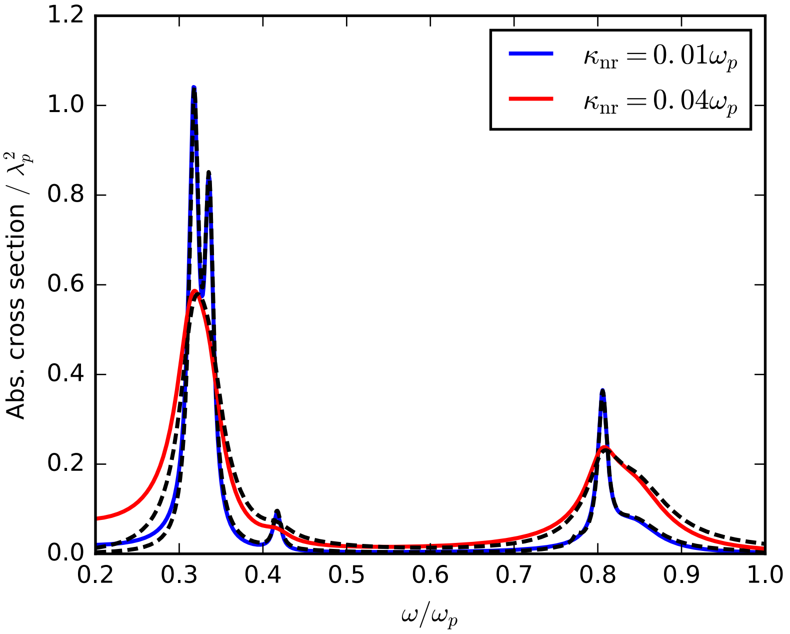


Figure S3. Absorption cross section of the multilayered spherical nanoparticle introduced in Sec. IID of the main text, for two different values of the Drude nonradiative dissipation rate. The solid curves are obtained with the quasinormal-mode expansion, whereas the dashed curves are computed from generalized Mie theory.
